# Supplementary material for: A Collective Learning Framework to Boost GNN Expressiveness
Source: arXiv:2003.12169 source file (2020-09-28)
Supplement: Supplementary file 1 [file appendix.tex]

\appendix
\section{Do \emph{not} have an appendix here}

\textbf{\emph{Do not put content after the references.}}
Put anything that you might normally include after the references in a separate
supplementary file.

We recommend that you build supplementary material in a separate document.
If you must create one PDF and cut it up, please be careful to use a tool that
doesn't alter the margins, and that doesn't aggressively rewrite the PDF file.
pdftk usually works fine. 

\textbf{Please do not use Apple's preview to cut off supplementary material.} In
previous years it has altered margins, and created headaches at the camera-ready
stage.

\subsection{Algorithms}

If you are using \LaTeX, please use the ``algorithm'' and ``algorithmic''
environments to format pseudocode. These require
the corresponding stylefiles, algorithm.sty and
algorithmic.sty, which are supplied with this package.
Algorithm~\ref{alg:example} shows an example.

\begin{algorithm}[tb]
   \caption{Bubble Sort}
   \label{alg:example}
\begin{algorithmic}
   \STATE {\bfseries Input:} data $x_i$, size $m$
   \REPEAT
   \STATE Initialize $noChange = true$.
   \FOR{$i=1$ {\bfseries to} $m-1$}
   \IF{$x_i > x_{i+1}$}
   \STATE Swap $x_i$ and $x_{i+1}$
   \STATE $noChange = false$
   \ENDIF
   \ENDFOR
   \UNTIL{$noChange$ is $true$}
\end{algorithmic}
\end{algorithm}

\begin{table}[t]
\caption{Classification accuracies for naive Bayes and flexible
Bayes on various data sets.}
\label{sample-table}
\vskip 0.15in
\begin{center}
\begin{small}
\begin{sc}
\begin{tabular}{lcccr}
\toprule
Data set & Naive & Flexible & Better? \\
\midrule
Breast    & 95.9$\pm$ 0.2& 96.7$\pm$ 0.2& $\surd$ \\
Cleveland & 83.3$\pm$ 0.6& 80.0$\pm$ 0.6& $\times$\\
Glass2    & 61.9$\pm$ 1.4& 83.8$\pm$ 0.7& $\surd$ \\
Credit    & 74.8$\pm$ 0.5& 78.3$\pm$ 0.6&         \\
Horse     & 73.3$\pm$ 0.9& 69.7$\pm$ 1.0& $\times$\\
Meta      & 67.1$\pm$ 0.6& 76.5$\pm$ 0.5& $\surd$ \\
Pima      & 75.1$\pm$ 0.6& 73.9$\pm$ 0.5&         \\
Vehicle   & 44.9$\pm$ 0.6& 61.5$\pm$ 0.4& $\surd$ \\
\bottomrule
\end{tabular}
\end{sc}
\end{small}
\end{center}
\vskip -0.1in
\end{table}
